# Supplementary material for: Algorithm for Optimized mRNA Design Improves Stability and Immunogenicity
Source: arXiv:2004.10177 source file (2022-03-17)

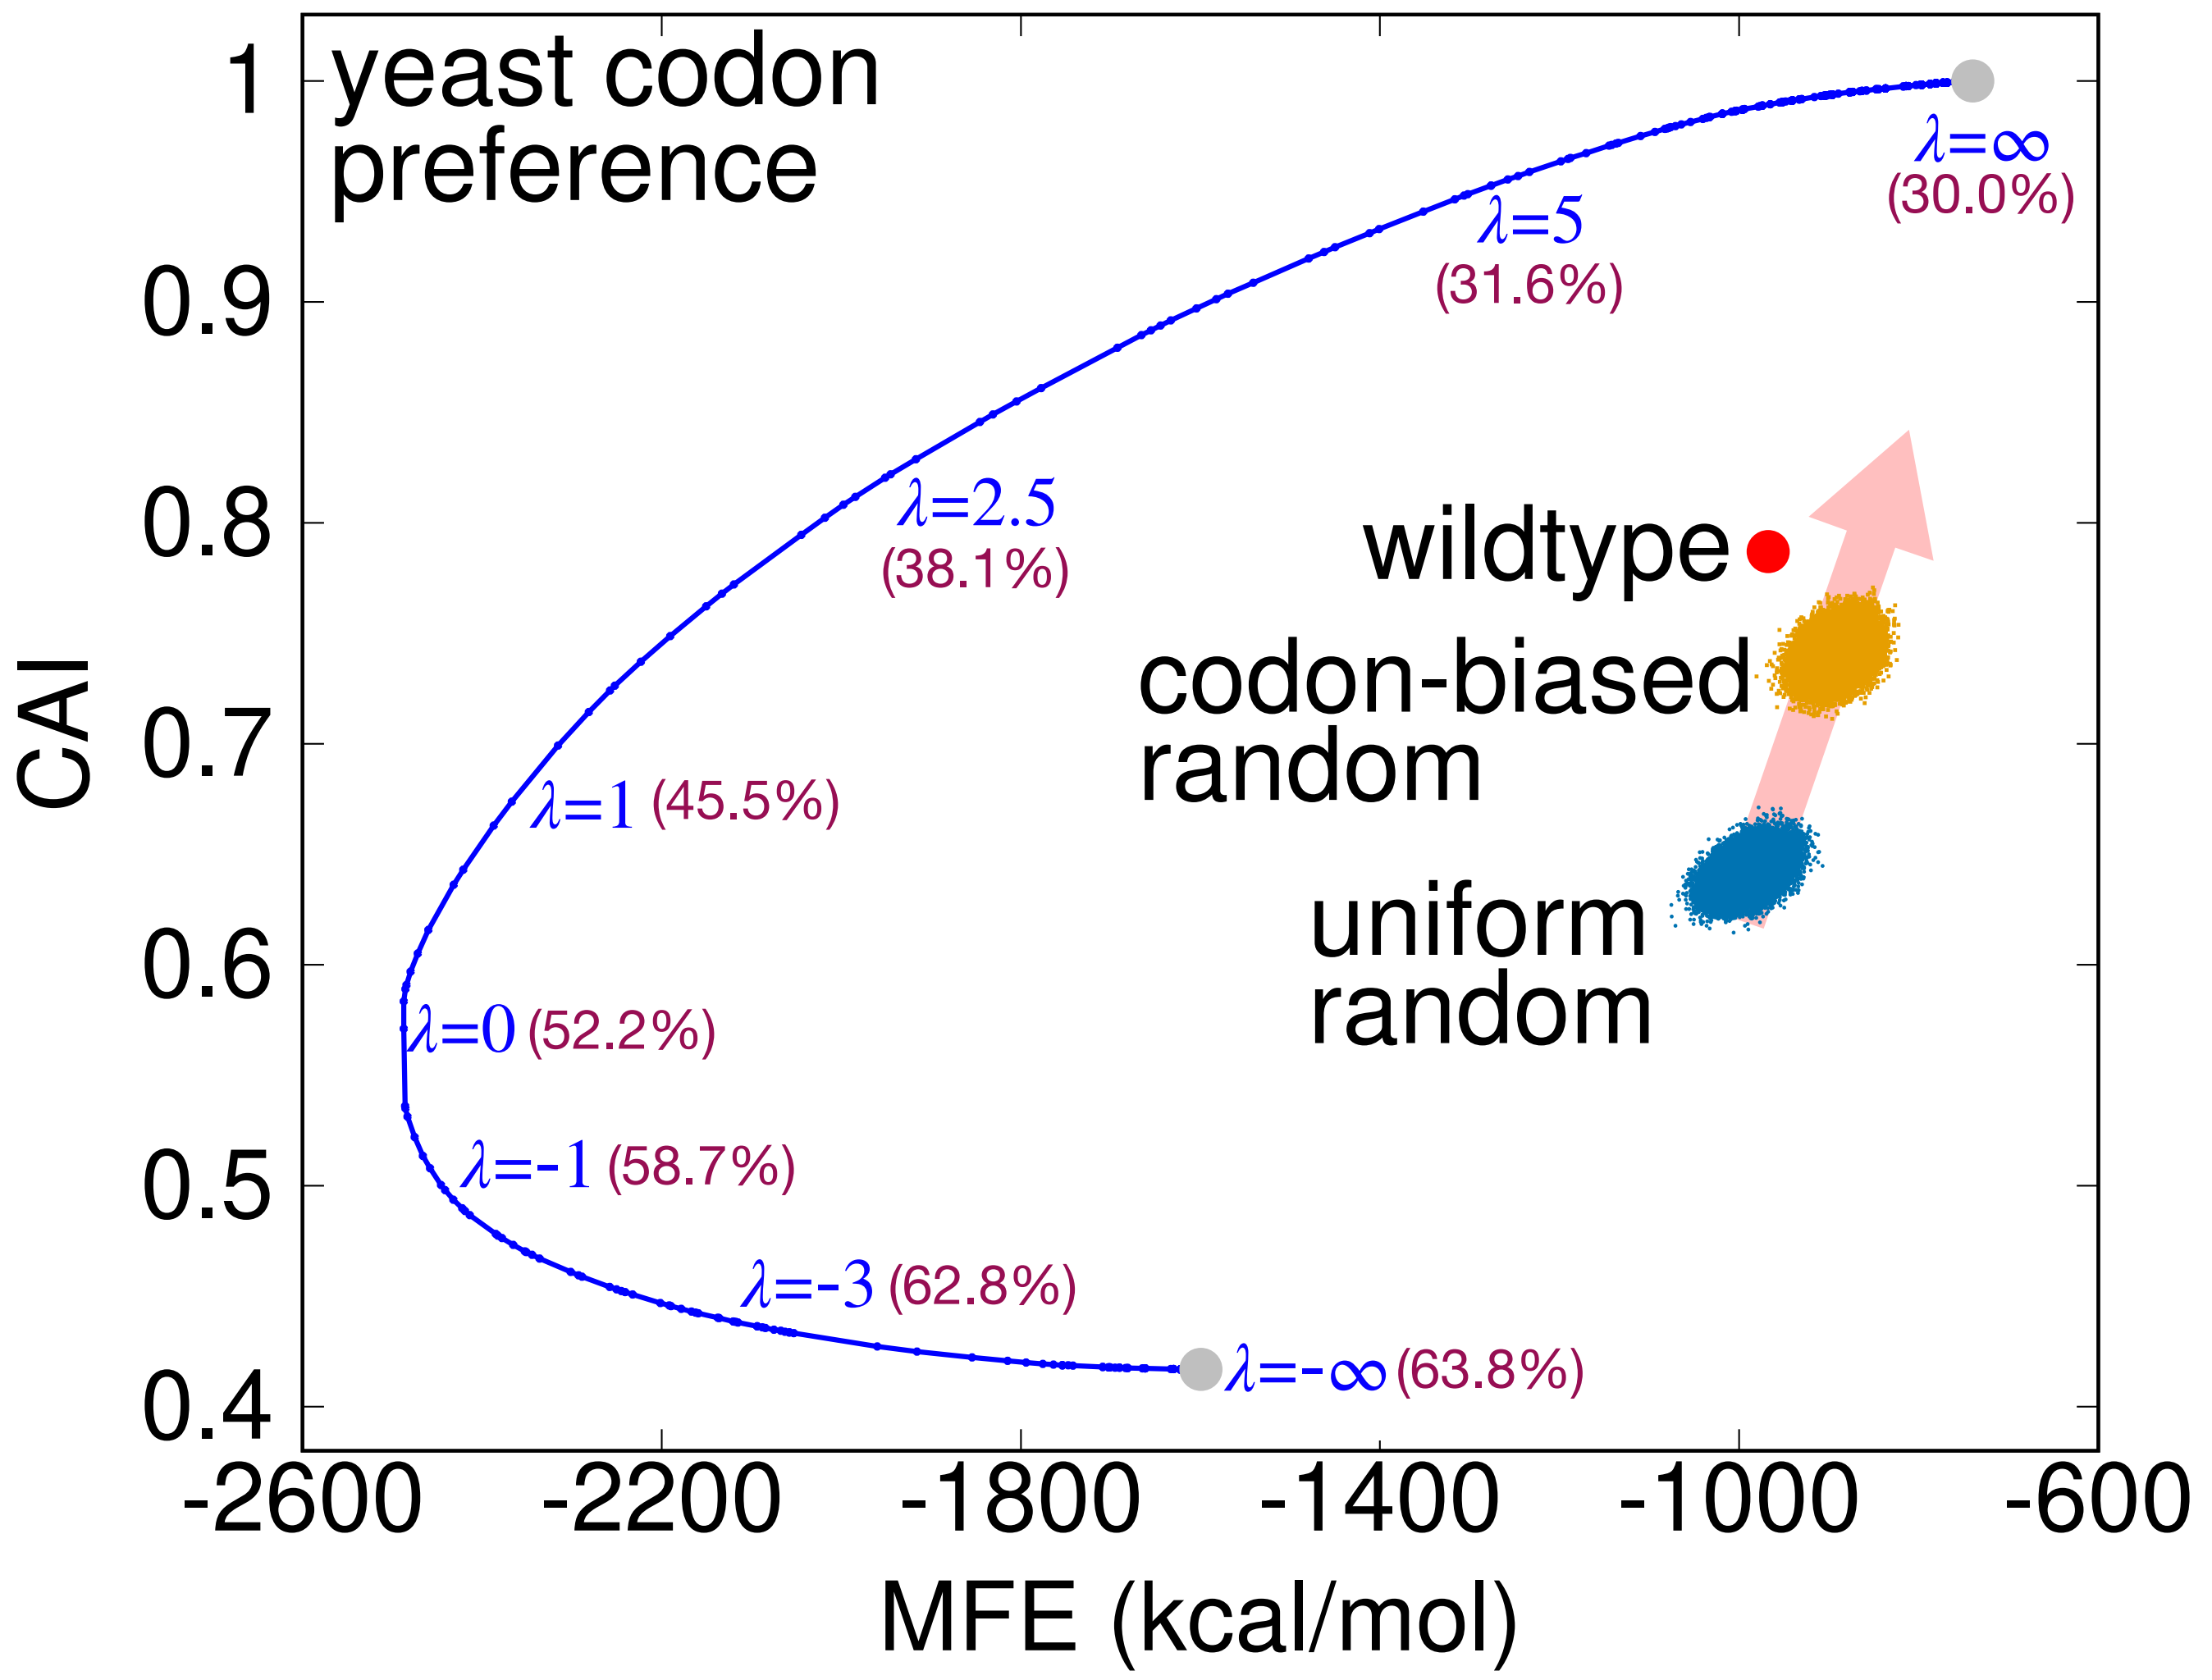

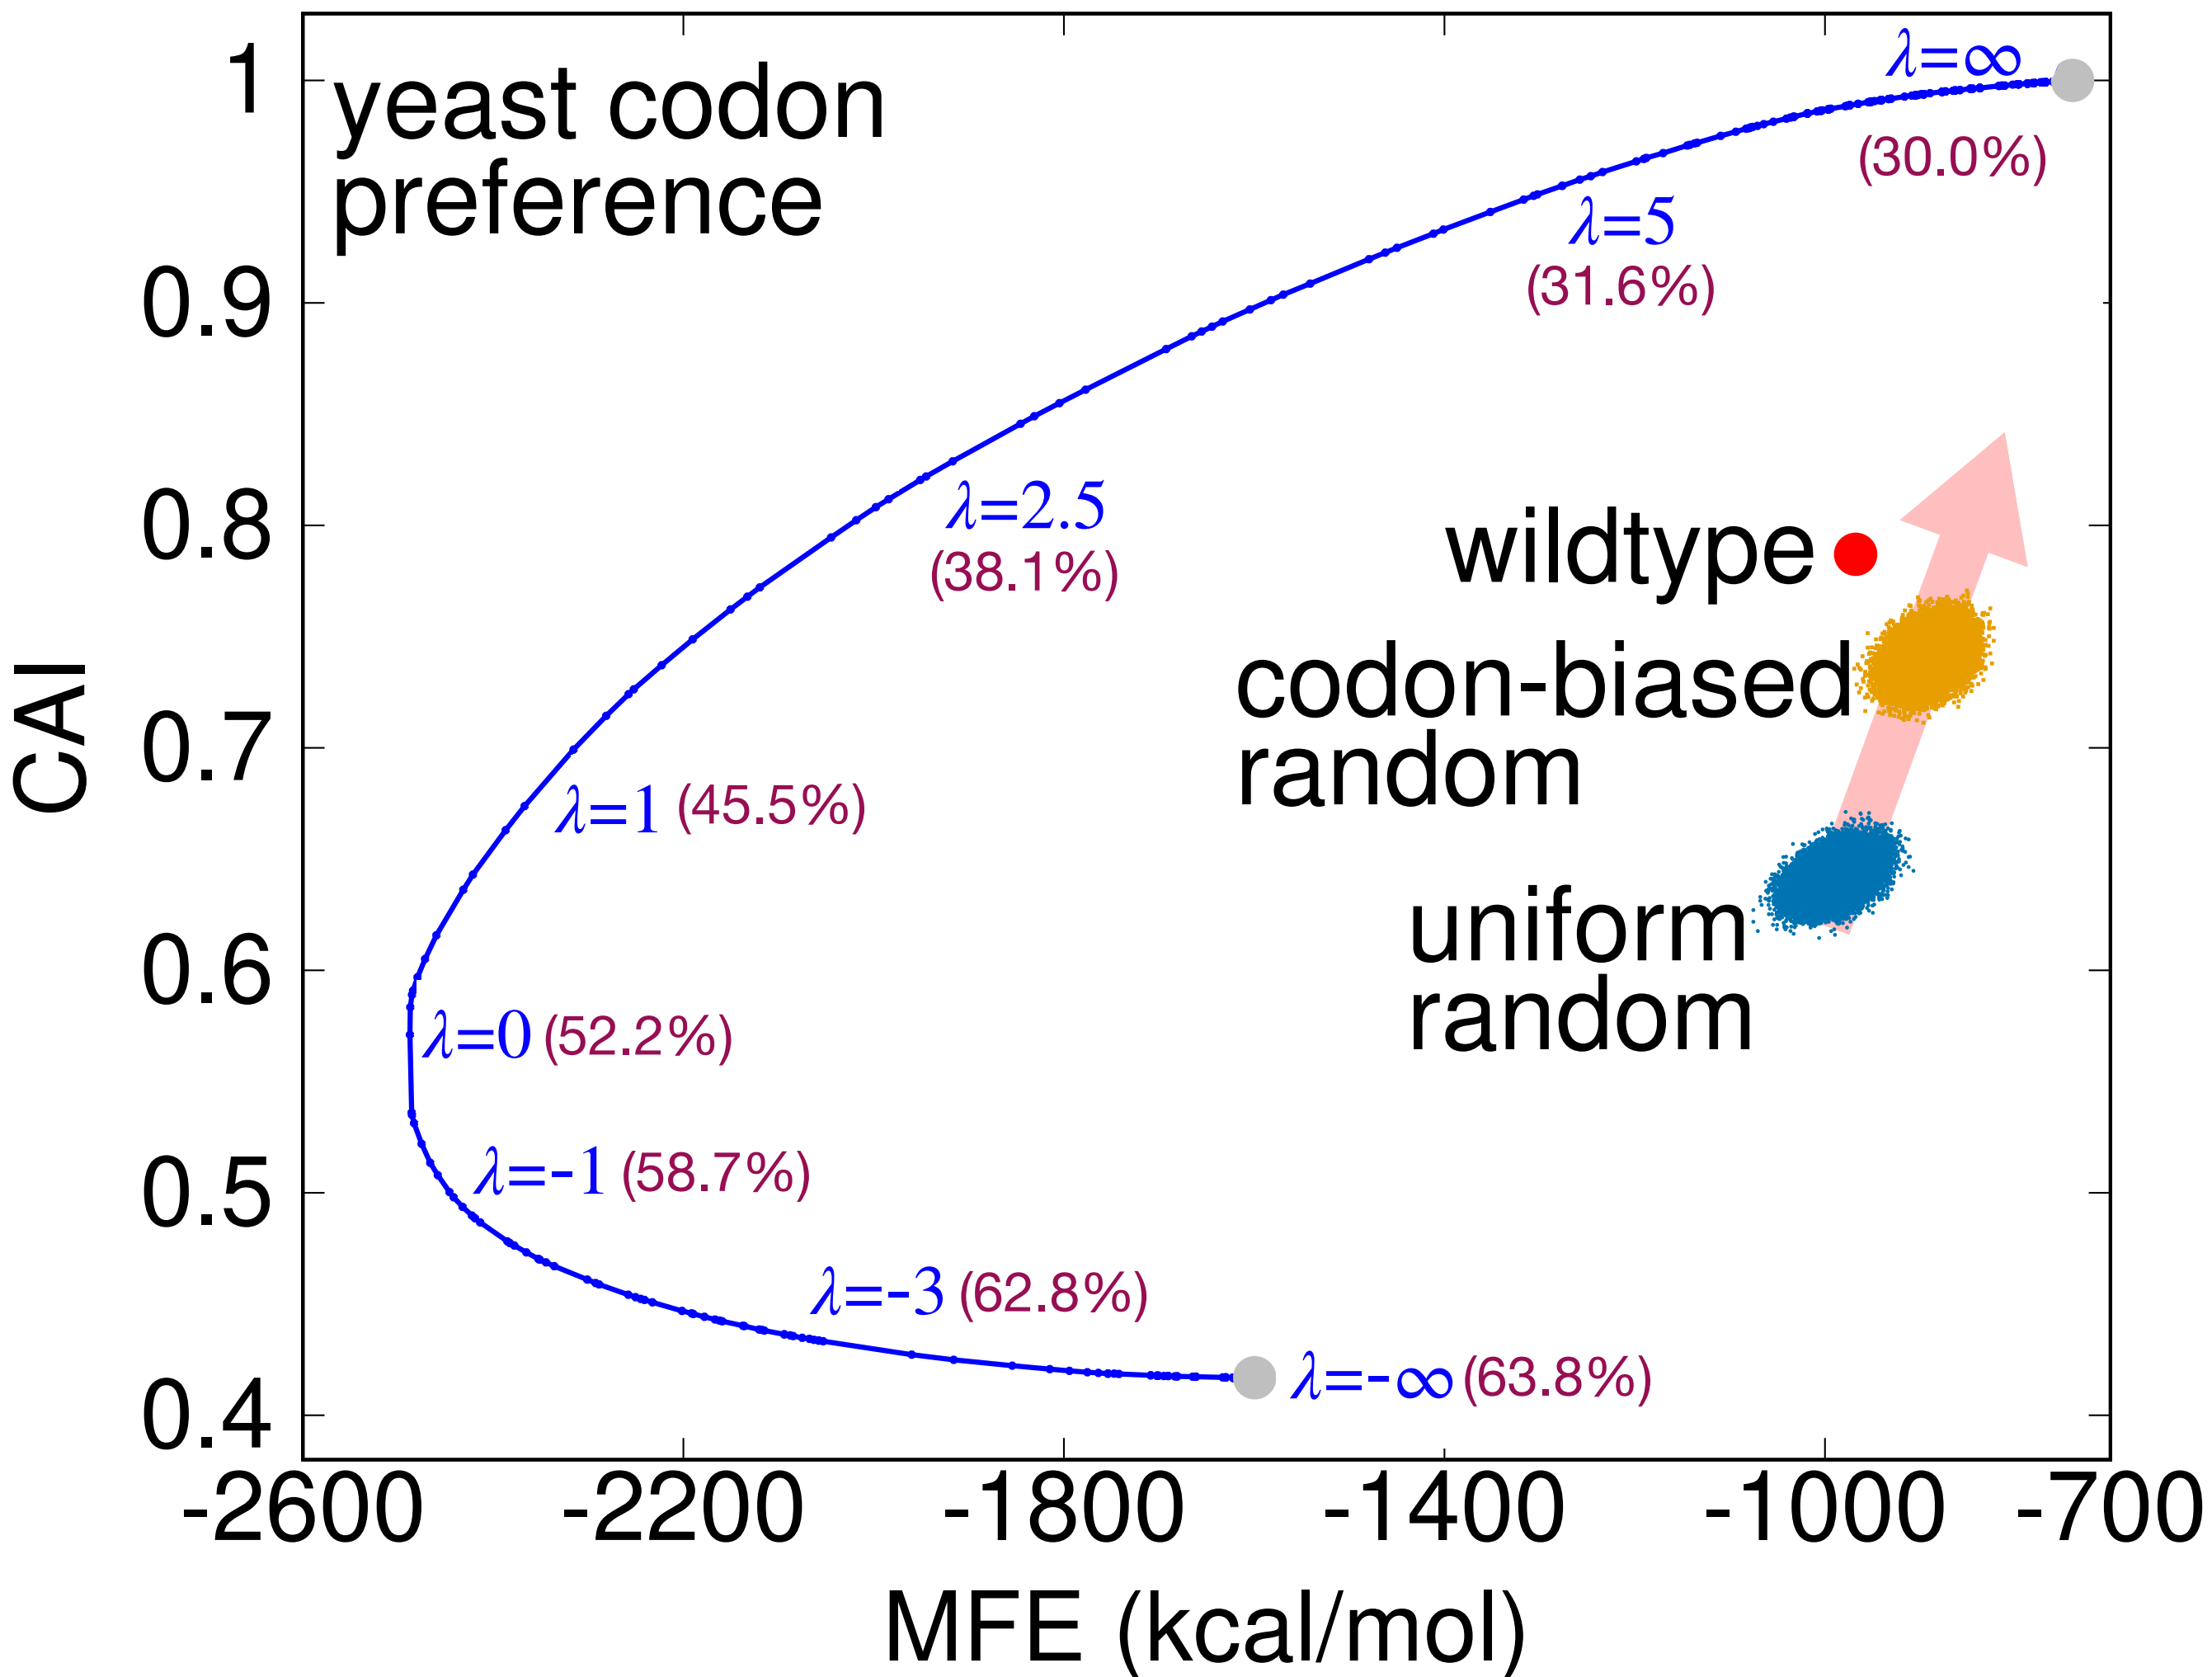

Supplement: Supplementary file 1 [file Spike_yeast_codon_oval_full.pdf]
